# Supplementary material for: Impact of the electronic band structure in high-harmonic generation spectra of solids
Source: arXiv:1609.09298 source file (2016-09-29)
Supplement: Supplementary file 1 [file SupMat.pdf]

# Impact of the electronic band structure in high-harmonic generation spectra of solids: supplementary material

Nicolas Tancogne-Dejean,[1,2,*] Oliver D. Mücke,[3,4] Franz X. Kärtner,[3,5,4,6] and Angel Rubio[1,2,3,5,†]
[1] *Max Planck Institute for the Structure and Dynamics of Matter, Luruper Chaussee 149, 22761 Hamburg, Germany*
[2] *European Theoretical Spectroscopy Facility (ETSF)*
[3] *Center for Free-Electron Laser Science CFEL, Deutsches Elektronen-Synchrotron DESY, Notkestraße 85, 22607 Hamburg, Germany*
[4] *The Hamburg Center for Ultrafast Imaging, Luruper Chaussee 149, 22761 Hamburg, Germany*
[5] *Physics Department, University of Hamburg, Luruper Chaussee 149, 22761 Hamburg, Germany*
[6] *Research Laboratory of Electronics, Massachusetts Institute of Technology, 77 Massachusetts Avenue, Cambridge, MA 02139, USA*

## COMPARISON OF THE JOINT DOS AND THE HHG SPECTRA FOR BULK ALAS

In order to show that our conclusions are valid not only for cubic silicon, we also performed calculations for bulk AlAs, which has a zinc-blende crystal structure. As this material does not have inversion symmetry, we expect odd and even harmonic peaks. We used a real-space spacing of 0.395 atomic units and an optimized 28×28×28 grid shifted four times to sample the BZ. The peak intensity inside matter is taken to be $I_0 = 10^{11}\,\mathrm{W\,cm^{-2}}$, and the carrier wavelength $\lambda$ is 3000 nm, corresponding to a carrier photon energy of 0.43 eV. The comparison between the joint DOS and the HHG spectra of AlAs is presented in Fig. 1.

As expected, we obtain that when the JDOS is low, the HHG exhibits clean harmonics, whereas higher JDOS is associated with noisy harmonics. Similarly to the case of bulk silicon, we see that the noisy region (orange shaded area) is suppressed, thus recovering clean odd and even harmonics (green shaded area), when the JDOS is very low.

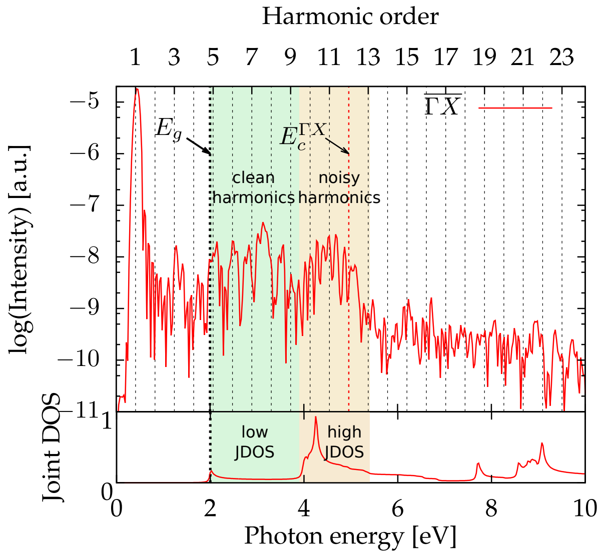


FIG. 1. HHG spectra for the $\overline{\Gamma X}$ polarization direction (red line). The bottom panel shows the corresponding joint DOS. The red and blue dashed lines indicate the position of the cutoff energy ($E_c$) for $\overline{\Gamma X}$. The shaded areas are guides to the eye.

## HHG SPECTRA AT HIGHER INTENSITY

We performed calculations at higher intensity $I_0 = 10^{12}\,\mathrm{W\,cm^{-2}}$. In order to get converged results, we employed a denser 38×38×38 grid shifted four times to sample the BZ.

As electrons explore a larger part of the Brillouin zone, the joint DOS is higher and no clean odd-harmonic structure is observed above the band gap, see Fig. 2.

We also note that the increase of the cutoff photon energy is consistent with a linear scaling in the electric field strength, as observed experimentally [1].

## EFFECT OF THE MATERIAL BAND GAP

In order to study the effect of the material band gap, we added in our time-dependent Kohn-Sham Hamiltonian a scissor operator, allowing us to artificially open the band gap by any value by shifting the conduction bands to higher energy. We have then simulated an artificial bulk silicon, increasing the band gap by 3.0 eV. We observe in Fig. 3 a region of clean odd-harmonics below the band gap, which is increased while increasing the band gap. This confirms once again that the interband contribution is suppressed for photon energies below the band gap. We also observe that the cutoff photon energy increases by the value of the bap opening ($\Delta = 3.0$ eV).

* nicolas.tancogne-dejean@mpsd.mpg.de
† angel.rubio@mpsd.mpg.de

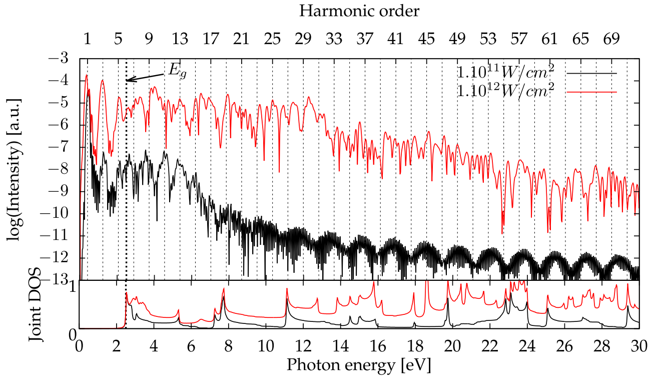


FIG. 2. Top panel: HHG spectra from bulk silicon computed within the local-density approximation, with laser polarization along the $\overline{\Gamma X}$ direction for $I_0 = 10^{11}\mathrm{W\,cm^{-2}}$ (black line) and $I_0 = 10^{12}\mathrm{W\,cm^{-2}}$ (red line). Bottom panel: Comparison of the joint DOS computed for the region explored by the electron for $I_0 = 10^{11}\mathrm{W\,cm^{-2}}$ (black line) and $I_0 = 10^{12}\mathrm{W\,cm^{-2}}$ (red line).

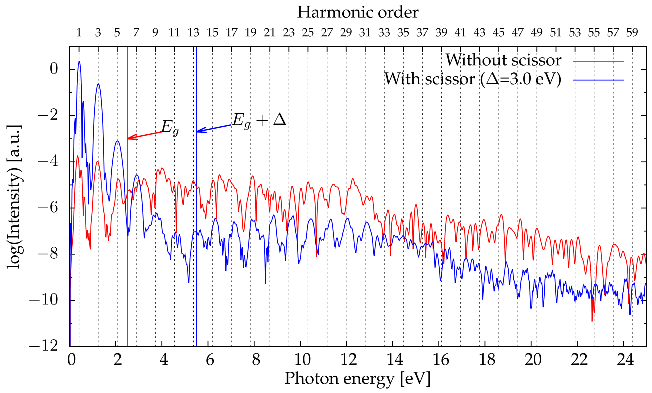


FIG. 3. HHG spectra from bulk silicon computed within the local-density approximation, with laser polarization along the Γ-X direction for $I_0 = 10^{12}\mathrm{W\,cm^{-2}}$, without scissor operator (red line) and including a scissor correction (Δ) of 3.0 eV (blue line).

[1] S. Ghimire, A. D. DiChiara, E. Sistrunk, P. Agostini, L. F. DiMauro, and D. A. Reis, Nature Physics **7**, 138 (2011).
